# Supplementary material for: On The Fragility of Learned Reward Functions
Source: arXiv:2301.03652 source file (2023-01-09)
Supplement: Supplementary file 1 [file appendix.tex]

\documentclass{article}

% if you need to pass options to natbib, use, e.g.:
%     \PassOptionsToPackage{numbers, compress}{natbib}
% before loading neurips_2022

% ready for submission
\usepackage[nonatbib]{neurips_2022}

% to compile a preprint version, e.g., for submission to arXiv, add add the
% [preprint] option:
%     \usepackage[preprint]{neurips_2022}

% to compile a camera-ready version, add the [final] option, e.g.:
%     \usepackage[final]{neurips_2022}

% to avoid loading the natbib package, add option nonatbib:
%    \usepackage[nonatbib]{neurips_2022}

\usepackage[utf8]{inputenc} % allow utf-8 input
\usepackage[T1]{fontenc}    % use 8-bit T1 fonts
\usepackage{hyperref}       % hyperlinks
\usepackage{url}            % simple URL typesetting
\usepackage{booktabs}       % professional-quality tables
\usepackage{amsfonts}       % blackboard math symbols
\usepackage{nicefrac}       % compact symbols for 1/2, etc.
\usepackage{microtype}      % microtypography
\usepackage{xcolor}         % colors
\usepackage{todonotes}      % todos
\usepackage{graphicx}       % allows us to include images
\usepackage{hyperref}
\usepackage[toc,page]{appendix}
\usepackage[square,numbers]{natbib}

% beginning of packages imported from the authors
\usepackage{comment}
% end of packages imported from the authors

\usepackage{dblfloatfix}

\bibliographystyle{abbrvnat}

\begin{document}

\bibliography{references}

\bibliography{references}
\end{document}
